# Supplementary material for: Flexible Tool Selection through Low-dimensional Attribute Alignment of Vision and Language
Source: arXiv:2505.22146 ancillary file (2025-08-21)
Supplement: Supplementary file 1 [file Supplementary_Material.pdf]

## Supplementary Material

## "Flexible Tool Selection through Low-dimensional Attribute Alignment of Vision and Language"

### Figures


| | | Page |
|---|---|---|
| Figure s-1 | Tool categories in the ToolNet dataset | 2 |
| Figure s-2 | Descriptions and rating criteria for all attributes | 3 |
| Figure s-3 | Prompting strategy for scenario generation | 4 |
| Figure s-4 | Sample task from the Tool Matching Dataset | 5 |

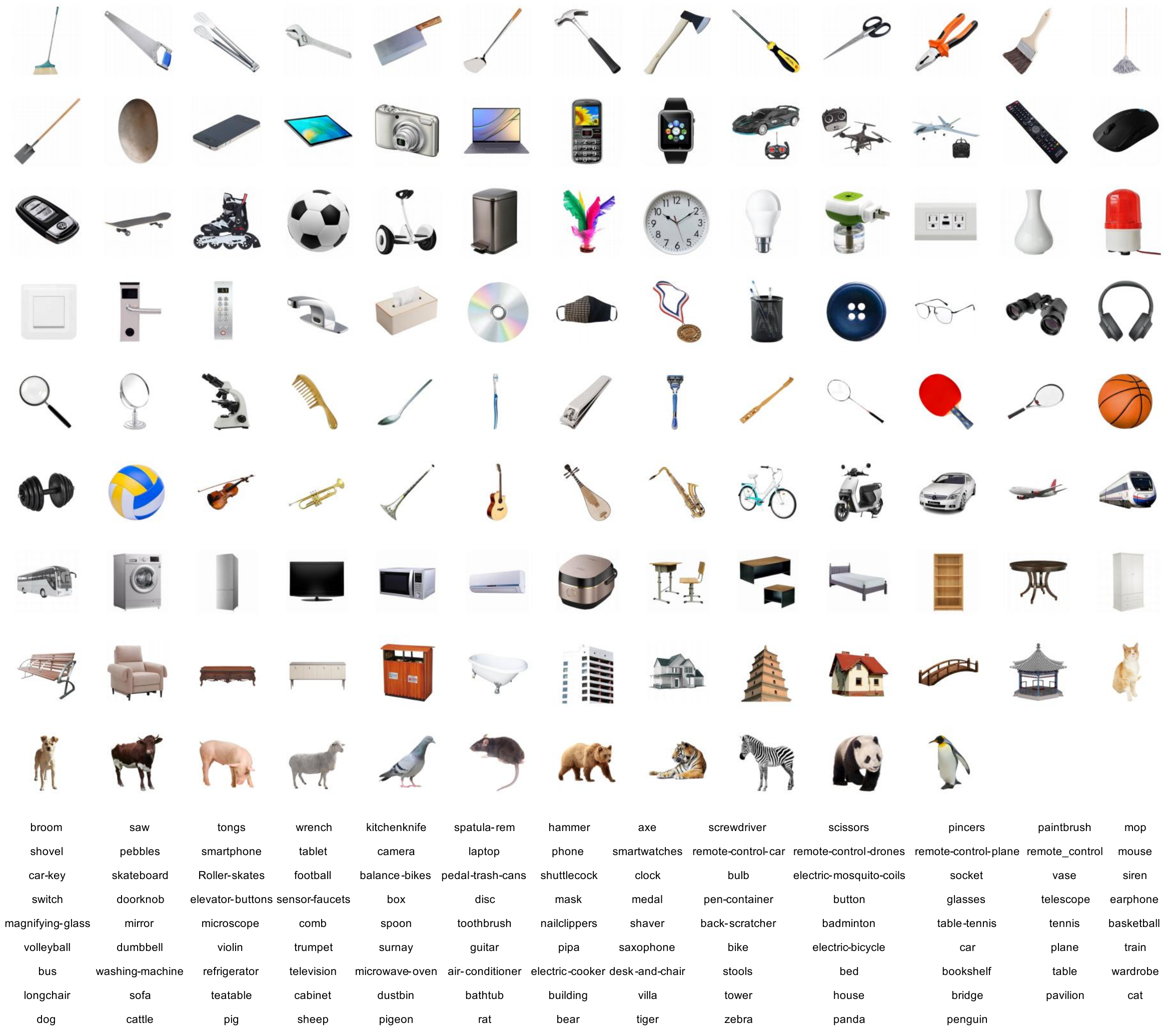


Figure s-1: **Tool categories in the ToolNet dataset.** Representative images and names for each of the 115 tool categories included in our study. Tools span diverse domains including kitchen implements, gardening equipment, workshop tools, and household items. Each category uses the same attribute vector derived from human ratings across all its image instances.

## Attribute Explanations

### Physical Attributes

**Elongation**
The degree to which the object is long and slender in shape. A rating of 7 indicates a very elongated object (like a baseball bat), while 1 indicates a non-elongated object (like a disc).

**Spiky**
The presence and prominence of protrusions or sharp points on the object. A rating of 7 indicates many prominent spikes or points (like a hedgehog), while 1 indicates no spikes or points (like a smooth disc).

**Size**
The physical size of the object in the real world. A rating of 7 indicates a very large object (like a car), while 1 indicates a very small object (like an ant).

**Smoothness**
The texture of the object's surface. A rating of 7 indicates a very rough surface (like tree bark), while 1 indicates a very smooth surface (like glass).

**Texturedness**
The complexity of patterns or textures on the object's surface. A rating of 7 indicates complex, irregular patterns (like floral fabric), while 1 indicates a uniform, simple surface (like a steel pipe).

**Hardness**
The physical hardness of the object's material. A rating of 7 indicates a very hard material that's difficult to deform (like an iron door), while 1 indicates a soft material easily changed in shape (like modeling clay).

### Interaction Attributes

**Graspability**
How easily the object can be picked up or grasped. A rating of 7 indicates an object that's very easy to grasp (like a broom), while 1 indicates an object that's difficult to grasp (like a tank).

**Hand**
The degree to which the object requires hand interaction during use. A rating of 7 indicates high hand involvement (like using darts), while 1 indicates low hand involvement (like dance shoes).

**Force**
The amount of physical effort or muscular activity required to use the object. A rating of 7 indicates high physical effort (like using a hoe), while 1 indicates minimal effort (like using an embroidery needle).

**Body**
How much the object feels like an extension of the user's body during use. A rating of 7 indicates the object feels like a body extension, while 1 indicates no sense of body extension (like a pond).

### Emotional Attributes

**Threatness**
The perceived level of danger associated with the object. A rating of 7 indicates a very dangerous object (like explosives), while 1 indicates a harmless object (like cotton).

**Valence**
The emotional response the object typically evokes. A rating of 7 indicates a very positive emotional response (like a trophy), while 1 indicates a very negative emotional response (like a corpse).

**Arousal**
The level of excitement or alertness the object typically induces. A rating of 7 indicates high arousal/excitement (like a bomb causing high alertness), while 1 indicates low arousal/calmness (like an eraser causing relaxation).

Figure s-2: **Descriptions and rating criteria for all attributes.** The attributes are categorized into three groups: physical properties, functional properties and psychological properties. Each dimension includes specific definitions, anchor points, and concrete examples to ensure consistent ratings across 30 participants using a 1-7 scale.

## Scene Generation Prompt Template

**System Prompt:**

You are a helpful assistant that generates realistic tool usage scenarios.

**User Prompt:**

You are helping to generate scenarios where tools are used. For the tool **"{tool_name}"**,
I will provide its properties and their ratings on a 1-7 scale. Each property has been rated by human evaluators based on specific criteria:

Tool Properties and Ratings:
- Elongation (Rating: **x.x**) : **{property_explanations[Elongation]}**
- Spiky (Rating: **x.x**) : **{property_explanations[Spiky]}**
- Size (Rating: **x.x**) : **{property_explanations[Size]}**
- Smoothness (Rating: **x.x**) : **{property_explanations[Smoothness]}**
- Texturedness (Rating: **x.x**) : **{property_explanations[Texturedness]}**
- Hardness (Rating: **x.x**) : **{property_explanations[Hardness]}**
- Graspability (Rating: **x.x**) : **{property_explanations[Graspability]}**
- Hand (Rating: **x.x**) : **{property_explanations[Hand]}**
- Force (Rating: **x.x**) : **{property_explanations[Force]}**
- Body (Rating: **x.x**) : **{property_explanations[Body]}**
- Threatness (Rating: **x.x**) : **{property_explanations[Threatness]}**
- Valence (Rating: **x.x**) : **{property_explanations[Valence]}**
- Arousal (Rating: **x.x**) : **{property_explanations[Arousal]}**

Based on these property ratings, generate **{num_to_generate}** different scenarios where this tool would naturally be used. Each scenario should be a single sentence describing the action and result, without mentioning the tool's name or explicitly describing its properties.

Remember to:
1. Keep scenarios concise but descriptive
2. Make scenarios realistic and practical
3. Vary the contexts and uses
4. Focus on the action and result (e.g., "The classroom floor was spotless after the morning cleaning" instead of "The janitor used a broom to sweep the floor")
5. Keep scenarios concise but vivid
6. Avoid mentioning the tool name
7. Write naturally without forcing property descriptions

Format your response as a JSON array of strings, like this:
["Scenario 1", "Scenario 2", ...]

Example good scenarios for a cleaning tool:
- Dust and crumbs disappeared from under the kitchen cabinets with a few quick motions
- The fallen autumn leaves were quickly cleared from the front porch
- Within minutes, the scattered rice grains were gathered into a neat pile

Figure s-3: **Prompting strategy for scenario generation.** Illustration of the detailed prompting strategy used for generating natural language descriptions of tool usage scenarios using Gemini-2.0-flash-experimental LLM.

**Task Scenario**

The forester thinned the trees, improving the health and growth of the remaining forest.

**Tools to be selected**

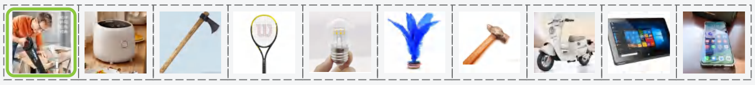

**deepseek-resnet50**

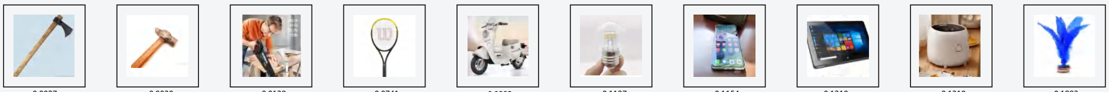


**Target rank: 3**

**ds_r1_qwen2_1.5b**

</think>\n\n1. Tool 3 (axe) \n2. Tool 1 (saw) \n3. Tool 4 (tennis) \n4. Tool 9 (tablet) \n5. Tool 2 (electric-cooker) \n6. Tool 8 (electric-bicycle) \n7. Tool 7 (hammer) \n8. Tool 5 (bulb) \n9. Tool 6 (shuttlecock) \n10. Tool 10 (smartphone)

**Target rank: 2**

**qwen2.5-vl-7b-instruct (STA)**

1. Tool 3\n2. Tool 7\n3. Tool 8\n4. Tool 6\n5. Tool 9\n6. Tool 10\n7. Tool 1\n8. Tool 2\n9. Tool 4\n10. Tool 5

**Target rank: 7**

**qwen2.5-vl-7b-instruct (CoT)**

### Step-by-Step Reasoning:\n\n1. **Understanding the Scenario**: The scenario describes a forester thinning trees, which involves cutting down or removing some trees to improve the health and growth of the remaining forest. This typically requires tools that can cut through wood effectively.\n\n2. **Analyzing Each Tool**:\n - **Tool 1 (Hand Saw)**: Suitable for cutting wood.\n - **Tool 2 (Electric Rice Cooker)**: Not suitable for cutting wood; used for cooking rice.\n - **Tool 3 (Axe)**: Suitable for cutting wood.\n - **Tool 4 (Tennis Racket)**: Not suitable for cutting wood; used for playing tennis.\n - **Tool 5 (LED Light Bulb)**: Not suitable for cutting wood; used for lighting.\n - **Tool 6 (Blue Feather)**: Not suitable for cutting wood; decorative item.\n - **Tool 7 (Hammer)**: Not suitable for cutting wood; used for hammering nails.\n - **Tool 8 (Scooter)**: Not suitable for cutting wood; used for transportation.\n - **Tool 9 (Tablet)**: Not suitable for cutting wood; used for computing.\n - **Tool 10 (Smartphone)**: Not suitable for cutting wood; used for communication and computing.\n\n3. **Ranking Based on Suitability**:\n - **Most Suitable Tools**: Hand saws and axes are the most relevant as they are designed for cutting wood.\n - **Least Suitable Tools**: All other tools are not related to cutting wood.\n\n### Final Response:\n\n1. Tool 3 (Axe)\n2. Tool 1 (Hand Saw)\n3. Tool 7 (Hammer) - slightly less relevant than an axe but still somewhat related\n4. Tool 8 (Scooter) - least relevant as it is not a tool for cutting wood\n5. Tool 9 (Tablet) - least relevant as it is not a tool for cutting wood\n6. Tool 10 (Smartphone) - least relevant as it is not a tool for cutting wood\n7. Tool 2 (Electric Rice Cooker) - least relevant as it is not a tool for cutting wood\n8. Tool 6 (Blue Feather) - least relevant as it is not a tool for cutting wood\n9. Tool 5 (LED Light Bulb) - least relevant as it is not a tool for cutting wood\n10. Tool 4 (Tennis Racket) - least relevant as it is not a tool for cutting wood

**Target rank: 2**

**Gemini-2.0 Pro (STA)**

1. Tool 3\n2. Tool 1\n3. Tool 7\n4. Tool 2\n5. Tool 4\n6. Tool 5\n7. Tool 6\n8. Tool 8\n9. Tool 9\n10. Tool 10\n

**Target rank: 2**

**Gemini-2.0 Pro (CoT)**

Okay, let's analyze the scenario and the tools. The scenario describes a forester thinning trees, which means selectively removing some trees to benefit the overall health of the forest. This requires tools for cutting or removing trees.\n\nHere's a breakdown of each tool and its suitability, followed by the final ranking:\n\n* **Tool 1 (Hand Saw):** This is a saw suitable for cutting wood. A hand saw is a viable, albeit labor-intensive, tool for felling smaller trees or branches. This is a good match.\n\n* **Tool 2 (Rice Cooker):** A rice cooker is for cooking rice. It has absolutely no relevance to forestry or tree thinning. This will rank very low.\n\n* **Tool 3 (Axe):** An axe is a classic tool for chopping wood and felling trees. It's a very direct and effective tool for the task, though it requires skill and effort. This is the best match.\n\n* **Tool 4 (Tennis Racket):** A tennis racket is used for playing tennis. It has no application in forestry. This will rank very low.\n\n* **Tool 5 (Light Bulb):** A light bulb provides light. While light *could* be useful in a forest (e.g., at night), it's not directly involved in the act of thinning trees. This is not relevant.\n\n* **Tool 6 (Shuttlecock):** Used for playing badminton, irrelevant for the scenerio.\n\n* **Tool 7 (Hammer):** Hammers are primarily for driving nails or breaking things. While a hammer *could* be used in forestry (e.g., to build something), it's not directly used for thinning trees. This will rank relatively low, but above completely irrelevant items.\n\n* **Tool 8 (Scooter):** A scooter is used for transportation, not applicable to the main task.\n\n* **Tool 9 (Tablet):** The tablet itself won't thin the tree, no relevance.\n\n* **Tool 10 (Smart Phone):** The smart phone has no direct use in thinning tree, rank low.\n\n**Final Ranking:**\n\n1. Tool 3 (Axe)\n2. Tool 1 (Hand Saw)\n3. Tool 7 (Hammer)\n4. Tool 5 (Light Bulb)\n5. Tool 8 (Scooter)\n6. Tool 9 (Tablet)\n7. Tool 10 (Smart Phone)\n8. Tool 4 (Tennis Racket)\n9. Tool 6 (Shuttlecock)\n10. Tool 2 (Rice Cooker)\n

**Target rank: 2**

**GPT-4o (STA)**

1. Tool 3\n2. Tool 1\n3. Tool 7\n4. Tool 8\n5. Tool 9\n6. Tool 10\n7. Tool 6\n8. Tool 4\n9. Tool 5\n10. Tool 2

**Target rank: 2**

**GPT-4o (CoT)**

To rank the tools based on the scenario \"The forester thinned the trees, improving the health and growth of the remaining forest,\" I need to determine which tools are most appropriate for thinning trees. Typically, tools like saws and axes are used for tasks like tree thinning.\n\nLet's analyze each tool image:\n\n1. **Tool 1**: This is an image of a saw, which is suitable for cutting wood and thinning trees.\n2. **Tool 2**: This is a rice cooker, which is unrelated to tree thinning.\n3. **Tool 3**: This is an axe, another tool well-suited for chopping trees and branches.\n4. **Tool 4**: A tennis racket, which is not useful for tree thinning.\n5. **Tool 5**: This is a light bulb, which is unrelated to tree thinning.\n6. **Tool 6**: This appears to be a traditional shuttlecock, which is unrelated to tree thinning.\n7. **Tool 7**: A hammer, which might be used in forestry but not primarily for tree thinning.\n8. **Tool 8**: A scooter, which is unrelated to tree thinning.\n9. **Tool 9**: A tablet, unrelated to tree thinning.\n10. **Tool 10**: A smartphone, also unrelated to tree thinning.\n\nGiven this analysis, the tools that directly relate to tree thinning (saw and axe) will rank highest, while those unrelated will rank lower.\n\nHere is the ranking:\n\n1. Tool 3 (Axe)\n2. Tool 1 (Saw)\n3. Tool 7 (Hammer - might have limited use in forestry work)\n4. Tool 2 (Rice Cooker - unrelated)\n5. Tool 4 (Tennis Racket - unrelated)\n6. Tool 5 (Light Bulb - unrelated)\n7. Tool 6 (Shuttlecock - unrelated)\n8. Tool 8 (Scooter - unrelated)\n9. Tool 9 (Tablet - unrelated)\n10. Tool 10 (Smartphone - unrelated)\n\nThis ranking reflects the relevance of the tools to the task of thinning trees.

**Target rank: 2**

Figure s-4: **Sample task from the Tool Matching Dataset.** This example showcases all model predictions for a sample task from the Tool Matching Dataset.
